# Supplementary material for: Self Model for Embodied Intelligence: Modeling Full-Body Human Musculoskeletal System and Locomotion Control with Hierarchical Low-Dimensional Representation
Source: arXiv:2312.05473 source file (2024-12-26)
Supplement: Supplementary file 1 [file Appendix.tex]

\onecolumn
\centerline{\huge Appendix}
~\

\section*{\large Body Segments, Joints, and Muscles}

The number of body segments in different body parts and their corresponding anatomical means are presented in Table. \ref{tab:body}. The pelvis serves as the root component of the kinematic tree. We have assigned appropriate mass and inertia properties to each body segment to facilitate dynamic simulation of the model.

\begin{table}[htbp]
  \centering
  \caption{Body Segments In Our Model}
  \begin{tabular}{ccc}
    \toprule
    Body Part & \makecell[c]{Number of \\Body Segments} & Anatomical Means           \\
    \midrule
    Pelvis & 1 & The base segment of kinematic tree \\
    \hline
    \makecell[c]{Lower \\Extremity} & 12 & \makecell[c]{Femurs, Patellas, Tibias/Fibulas, \\ Taluses, Calcanei and Toes} \\
    \hline
    Torso & 55 &\makecell[c]{Lumbosacral Symphysis, \\Joints of Vertebral Column, Costovertebral Joints}\\
    \hline
    \makecell[c]{Upper \\Extremity} & 22 & \makecell[c]{Clavicles, Scapulas, Humeri, Ulnas, Radiuses, Carpi and Hands, \\ The phantom bodies of Clavicles, Scapulas, Humeri}\\
    \hline
    Total & 90                             \\
    \bottomrule
  \end{tabular}
  \label{tab:body}
\end{table}

The intricate nature of human joint motion, which often encompasses both rotation and translation of the axis of rotation\cite{klamroth-marganska_three-dimensional_2014}, necessitates the inclusion of phantom segments with minimal mass and non-shape properties\cite{saul2015benchmarking}. These segments allow for additional rotation and translation axes to be attached to them in the form of joints, particularly in the upper extremity model. The number of Joints of the body parts is listed in Table. \ref{tab:joint}.

\begin{table}[htbp]
  \centering
  \caption{Joints In Our Model}
  \begin{tabular}{ccc}
    \toprule
    Body Part & Number of Joints & Anatomical Means           \\
    \midrule
    Pelvis & 6 & The DOFs between the base segment and ground   \\
    \hline
    \makecell[c]{Lower \\Extremity} & 28 & \makecell[c]{Hip, Knee, Ankle, Metatarsophalangeal and Patellofemoral Joints, \\Translation and rotation of the tibia and patella relative to the femur}   \\
    \hline
    Torso & 132 &  \makecell[c]{Lumbosacral Symphysis, Joints of Vertebral Column, Costovertebral Joints}\\
    \hline
    \makecell[c]{Upper \\Extremity} & 40 & \makecell[c]{Sternoclavicular, Acromioclavicular, Shoulder Joints, \\ Humeroulnar, Radioulnar, Radiocarpal, Carpometacarpal Joints}\\
    \hline
    Total & 206                              \\
    \bottomrule
  \end{tabular}
  \label{tab:joint}
\end{table}

As shown in Table.\ref{tab:muscle}, the full-body musculoskeletal model has 700 muscle-tendon units that act as skeletal muscles, applying pulling forces to bones to move joints. If a muscle has a large number of attachment points with body parts anatomically, such as the psoas in Fig. \ref{fig:sim_a}, it is modeled as multiple independent muscle-tendon units as in Fig. \ref{fig:sim_b}. Hence, the total number of muscle-tendon units (700) in our model surpasses the conventional estimation of skeletal muscle count (approximately 640).

\begin{table}[htbp]
  \centering
  \caption{Muscles In Our Model}
  \begin{tabular}{ccc}
    \toprule
    Body Part & Muscle Group & \makecell[c]{Number of \\Muscle-tendon Units}           \\
    \midrule
    \multirow{3}{*}{\makecell[c]{Pelvis and \\Lower Extremity}} 
    &  Iliac and Gluteal Region &  46  \\
    &  Thigh &  32\\
    &  Calf &  22\\
    \hline
    \multirow{6}{*}{Torso} 
    &  Abdomen &  98\\
    &  Spinalis &  154\\
    &  Cervical &  38\\
    &  Thoracic &  26\\
    &  Lumbar &  38\\
    &  Intercostal &  152\\
    \hline
    \multirow{4}{*}{\makecell[c]{Upper \\Extremity}}
    &  Shoulder &  24\\
    &  Elbow &  18\\
    &  Forearm &  16\\
    &  Wrist/Hand &  36\\
    \hline
    Total & & 700                             \\
    \bottomrule
  \end{tabular}
  \label{tab:muscle}
\end{table}
